# Supplementary material for: Implications from ${B\to K^*\ell^+\ell^-}$ observables using $3 \text{fb}^{-1}$ of LHCb data
Source: arXiv:1506.04535 ancillary file (2017-01-27)
Supplement: Supplementary file 1 [file Supplementary.pdf]

**Supplementary material for  
“Implications from  $B \rightarrow K^* \ell^+ \ell^-$  observables using  $3 \text{ fb}^{-1}$  of LHCb data.”**

Rusa Mandal<sup>\*</sup> and Rahul Sinha<sup>†</sup>

*The Institute of Mathematical Sciences, Taramani, Chennai 600113, India*

(Dated: March 31, 2016)

In this note we present the supplementary material referred to in the main paper. For the convenience of the reader some details already presented in a previous paper ( Ref. [1]) are repeated here. In order to focus attention to the main points such material is present in shaded boxes with blue text. The essential inputs required as supplementary material are in normal text.

---

<sup>\*</sup> rusam@imsc.res.in

<sup>†</sup> sinha@imsc.res.in

# I. EXTRACTION OF $\varepsilon_\lambda$ FROM DATA.

In Ref. [1] it was shown that in the massless lepton limit the the most general parametric form of standard model amplitude for  $B \rightarrow K^* \ell^+ \ell^-$  decay is described in terms of six transversity amplitudes which can be written in the most general form as,

$$\mathcal{A}_\lambda^{L,R} = C_{L,R}^\lambda \mathcal{F}_\lambda - \tilde{\mathcal{G}}_\lambda = (\tilde{C}_9^\lambda \mp C_{10}) \mathcal{F}_\lambda - \tilde{\mathcal{G}}_\lambda. \quad (1)$$

This form of the amplitude comprehensively takes into account all contributions within it. The form includes all short-distance and long-distance effects, factorizable and nonfactorizable contributions, resonance contributions and complete electromagnetic corrections to hadronic operators up to all orders.

It should be noted that  $\mathcal{F}_\lambda$ 's and  $C_{10}$  are completely real in the SM, with all imaginary contributions to the amplitude arising only from the imaginary part of complex  $\tilde{C}_9^\lambda$  and  $\tilde{\mathcal{G}}_\lambda$  terms. Thus with the introduction of two variables  $r_\lambda$  and  $\varepsilon_\lambda$  the amplitude  $\mathcal{A}_\lambda^{L,R}$  in Eq. (1) can be rewritten as,

$$\mathcal{A}_\lambda^{L,R} = (\mp \hat{C}_{10} - r_\lambda) \mathcal{F}_\lambda + i\varepsilon_\lambda, \quad (2)$$

where,

$$r_\lambda = \frac{\text{Re}(\tilde{\mathcal{G}}_\lambda)}{\mathcal{F}_\lambda} - \text{Re}(\tilde{C}_9^\lambda), \quad (3)$$

$$\varepsilon_\lambda = \text{Im}(\tilde{C}_9^\lambda) \mathcal{F}_\lambda - \text{Im}(\tilde{\mathcal{G}}_\lambda). \quad (4)$$

In Ref. [1] it was shown how a complex contributions  $\varepsilon_\lambda$  to the amplitude of the decay mode  $B \rightarrow K^* \ell^+ \ell^-$ , can be taken into consideration. It was also shown how the  $\varepsilon_\lambda$  can be solved in terms of iterative solutions proportional to the observables  $A_7$ ,  $A_8$ ,  $A_9$  and a form factor ratio  $P_1$ . The expressions for all the three  $\varepsilon_\lambda$ 's are shown in Eqs. (76)–(78) of Ref. [1]. They are reproduced here for convenience.

$$\varepsilon_\perp = \frac{\sqrt{2}\pi\Gamma_f}{(r_0 - r_\parallel)\mathcal{F}_\perp} \left[ \frac{A_9 P_1}{3\sqrt{2}} + \frac{A_8 P_2}{4} - \frac{A_7 P_1 P_2 r_\perp}{3\pi \hat{C}_{10}} \right], \quad (5)$$

$$\varepsilon_\parallel = \frac{\sqrt{2}\pi\Gamma_f}{(r_0 - r_\parallel)\mathcal{F}_\perp} \left[ \frac{A_9 r_0}{3\sqrt{2}r_\perp} + \frac{A_8 P_2 r_\parallel}{4P_1 r_\perp} - \frac{A_7 P_2 r_\parallel}{3\pi \hat{C}_{10}} \right], \quad (6)$$

$$\varepsilon_0 = \frac{\sqrt{2}\pi\Gamma_f}{(r_0 - r_\parallel)\mathcal{F}_\perp} \left[ \frac{A_9 P_1 r_0}{3\sqrt{2}P_2 r_\perp} + \frac{A_8 r_\parallel}{4r_\perp} - \frac{A_7 P_1 r_0}{3\pi \hat{C}_{10}} \right]. \quad (7)$$

A point to be noted and explained in detail in Ref. [1] is that the  $(\varepsilon_\lambda/\Gamma_f^{1/2})$ 's are completely expressed in terms of observables and the form factor ratio  $P_1$ . However, these solutions are essentially iterative, since the  $r_\lambda$ 's and  $\hat{C}_{10}$  are derived in terms of the primed observables that depend on  $\varepsilon_\lambda$ . If the  $(\varepsilon_\lambda/\Gamma_f^{1/2})$  are small as should be expected, accurate solutions for them can be found with a few iterations. In Ref. [1] the variation of  $\varepsilon_\lambda$  with  $P_1$  was studied for  $1\text{fb}^{-1}$  LHC data and it was found that the solutions are not sensitive to the value of  $P_1$ .

We generate a set of events for every bin, with each event consisting of randomly chosen values drawn from Gaussian distributions generated for each of the observables  $F_L$ ,  $F_\perp$ ,  $A_4$ ,  $A_5$ ,  $A_{\text{FB}}$ ,  $A_7$ ,  $A_8$  and  $A_9$ . The distributions are generated using experimental results from Ref. [2], with the experimentally measured value as mean and the uncertainty as standard deviation.

$\varepsilon_\lambda$  are solved iteratively for every set of observables. We find converged iterative solutions for  $\varepsilon_\lambda/\sqrt{\Gamma_f}$  for each set of observables with the histograms shown in Fig. 1. The red (dark), light brown

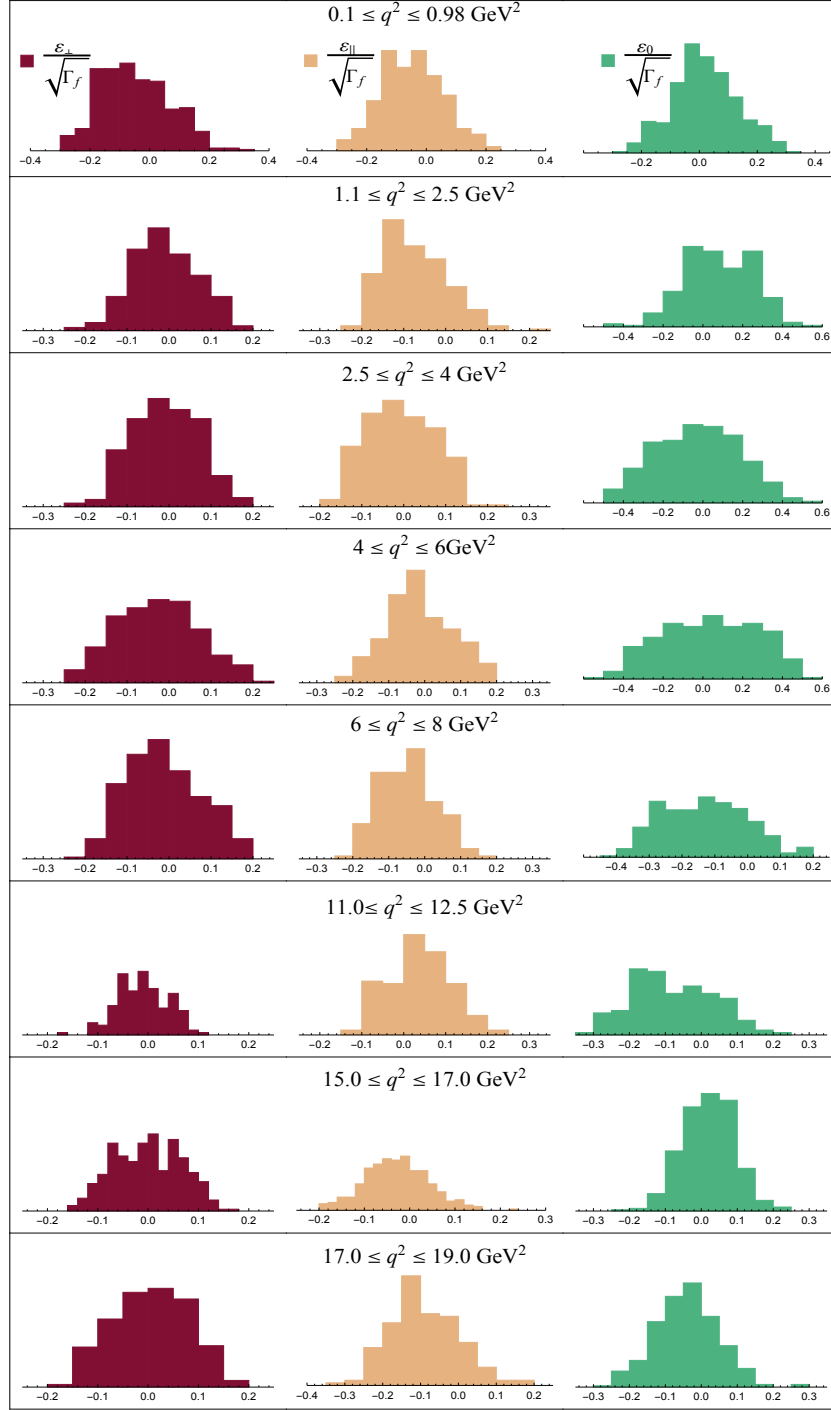

FIG. 1. The solutions for  $\varepsilon_{\perp}/\sqrt{\Gamma_f}$ ,  $\varepsilon_{\parallel}/\sqrt{\Gamma_f}$  and  $\varepsilon_0/\sqrt{\Gamma_f}$  using distributions for first through eighth  $q^2$  bins are depicted in red (dark), light brown (lightest) and green respectively. All the  $\varepsilon_{\lambda}/\sqrt{\Gamma_f}$ 's are consistent with zero.

(lightest) and green histograms denote the solutions for  $\varepsilon_{\perp}/\sqrt{\Gamma_f}$ ,  $\varepsilon_{\parallel}/\sqrt{\Gamma_f}$  and  $\varepsilon_0/\sqrt{\Gamma_f}$  respectively for all the eight bins with  $q^2$  range  $(0.1-0.98)$   $\text{GeV}^2$ ,  $(1.1-2.5)$   $\text{GeV}^2$ ,  $(2.5-4.0)$   $\text{GeV}^2$ ,  $(4-6)$   $\text{GeV}^2$ ,  $(6-8)$   $\text{GeV}^2$ ,  $(11.0-12.5)$   $\text{GeV}^2$ ,  $(15-17)$   $\text{GeV}^2$  and  $(17-19)$   $\text{GeV}^2$ .

We have also quoted the mean and  $1\sigma$  errors for each  $\varepsilon_{\lambda}/\sqrt{\Gamma_f}$  in Table. I calculated from the distributions shown in Fig. 1. It can be easily seen that all the mean values of  $\varepsilon_{\lambda}/\sqrt{\Gamma_f}$  are consistent

with zero. From Eqs. (37)–(40) of Ref. [1], the contributions from imaginary part of the amplitude to the observables  $F_L$ ,  $F_{\parallel}$ ,  $F_{\perp}$  and  $A_4$  are quadratic in the corresponding  $\varepsilon_{\lambda}/\sqrt{\Gamma_f}$  and thus are negligible.

| $q^2$ range in $\text{GeV}^2$ | $\varepsilon_{\perp}/\sqrt{\Gamma_f}$ | $\varepsilon_{\parallel}/\sqrt{\Gamma_f}$ | $\varepsilon_0/\sqrt{\Gamma_f}$ |
|-------------------------------|---------------------------------------|-------------------------------------------|---------------------------------|
| $0.1 \leq q^2 \leq 0.98$      | $-0.048 \pm 0.116$                    | $-0.047 \pm 0.103$                        | $0.020 \pm 0.111$               |
| $1.1 \leq q^2 \leq 2.5$       | $-0.010 \pm 0.078$                    | $-0.010 \pm 0.078$                        | $0.078 \pm 0.172$               |
| $2.5 \leq q^2 \leq 4.0$       | $-0.009 \pm 0.079$                    | $-0.008 \pm 0.080$                        | $-0.025 \pm 0.212$              |
| $4.0 \leq q^2 \leq 6.0$       | $-0.026 \pm 0.097$                    | $0.014 \pm 0.093$                         | $0.032 \pm 0.234$               |
| $6.0 \leq q^2 \leq 8.0$       | $-0.011 \pm 0.088$                    | $-0.046 \pm 0.078$                        | $-0.132 \pm 0.129$              |
| $11.0 \leq q^2 \leq 12.5$     | $-0.011 \pm 0.050$                    | $0.038 \pm 0.074$                         | $-0.078 \pm 0.114$              |
| $15.0 \leq q^2 \leq 17.0$     | $-0.0003 \pm 0.067$                   | $-0.027 \pm 0.071$                        | $0.020 \pm 0.072$               |
| $17.0 \leq q^2 \leq 19.0$     | $0.006 \pm 0.076$                     | $-0.090 \pm 0.090$                        | $-0.040 \pm 0.088$              |

TABLE I. The  $\varepsilon_{\lambda}/\sqrt{\Gamma_f}$  mean values with  $1\sigma$  errors from Fig. 1

## II. DETAILS ON THE DERIVATION OF EQS. (9)–(13).

As shown in Sec. IV of Ref. [1], neglecting  $\varepsilon_{\lambda}$  the observables  $F_L$ ,  $F_{\parallel}$ ,  $F_{\perp}$ ,  $A_4$ ,  $A_5$ ,  $A_{\text{FB}}$ ,  $A_7$ ,  $A_8$  and  $A_9$  can be expressed in terms of  $C_{10}$ ,  $r_{\lambda}$  and  $\mathcal{F}_{\lambda}$  as follows:

$$F_L \Gamma_f = 2 \frac{\mathcal{F}_{\perp}^2}{\mathbf{P}_2^2} (r_0^2 + C_{10}^2), \quad (8)$$

$$F_{\parallel} \Gamma_f = 2 \frac{\mathcal{F}_{\perp}^2}{\mathbf{P}_1^2} (r_{\parallel}^2 + C_{10}^2), \quad (9)$$

$$F_{\perp} \Gamma_f = 2 \mathcal{F}_{\perp}^2 (r_{\perp}^2 + C_{10}^2), \quad (10)$$

$$\sqrt{2} \pi A_4 \Gamma_f = 4 \frac{\mathcal{F}_{\perp}^2}{\mathbf{P}_1 \mathbf{P}_2} (r_0 r_{\parallel} + C_{10}^2), \quad (11)$$

$$\sqrt{2} A_5 \Gamma_f = 3 \frac{\mathcal{F}_{\perp}^2}{\mathbf{P}_2} C_{10} (r_0 + r_{\perp}), \quad (12)$$

$$A_{\text{FB}} \Gamma_f = 3 \frac{\mathcal{F}_{\perp}^2}{\mathbf{P}_1} C_{10} (r_{\parallel} + r_{\perp}) \quad (13)$$

Substituting for  $C_{10}$  and  $r_{\lambda}$  in terms  $\zeta$  and  $u_{\lambda}$  defined as follows:

$$\zeta = \frac{\mathcal{F}_{\perp}^2 C_{10}^2}{\Gamma_f}, \quad (14)$$

$$u_{\lambda}^2 = \frac{2 \mathcal{F}_{\perp}^2 r_{\lambda}^2}{\Gamma_f} = \frac{2}{\Gamma_f} \frac{\mathcal{F}_{\perp}^2}{\mathcal{F}_{\lambda}^2} \left( \text{Re}(\tilde{\mathcal{G}}_{\lambda}) - \text{Re}(\tilde{C}_9^{\lambda}) \mathcal{F}_{\lambda} \right)^2. \quad (15)$$

the desired equations can be derived easily.

### III. LEPTON MASS EFFECTS.

In Ref [1] it was shown how the corrections due to the mass of the leptons are easily taken into account. In the case of massive leptons there exists one more amplitude [5]

$$\mathcal{A}_t = \frac{2N}{\sqrt{q^2}} \lambda^{1/2} (m_B^2, m_{K^*}^2, q^2) C_{10} A_0(q^2) \quad (16)$$

In Sec. V of Ref [1] it was shown that the lepton mass effects can easily be included by redefining

$$\Gamma_f F_L \rightarrow \beta^2 \Gamma_f F_L + \mathbb{T}_1 \quad (17)$$

$$\Gamma_f F_{\parallel} \rightarrow \beta^2 \Gamma_f F_{\parallel} + \mathbb{T}_1 \quad (18)$$

$$\Gamma_f F_{\perp} \rightarrow \beta^2 \Gamma_f F_{\perp} + \mathbb{T}_1 \quad (19)$$

$$A_4 \rightarrow \beta^2 A_4 \quad (20)$$

$$A_5^2 \rightarrow \beta^2 A_5^2 \quad (21)$$

$$A_{\text{FB}}^2 \rightarrow \beta^2 A_{\text{FB}}^2 \quad (22)$$

$$A_7^2 \rightarrow \beta^2 A_7^2 \quad (23)$$

$$A_8 \rightarrow \beta^2 A_8 \quad (24)$$

$$A_9 \rightarrow \beta^2 A_9 \quad (25)$$

$$(26)$$

In the above we have defined

$$\mathbb{T}_1 = (|\mathcal{A}_t|^2 + \sum_{\lambda=\{\parallel, \perp, 0\}} |\mathcal{A}_{\lambda}^L + \mathcal{A}_{\lambda}^R|^2) \frac{m^2}{q^2} \quad (27)$$

$$= \frac{\Gamma_f}{3} - \frac{16}{9} A_{10} + \frac{64}{27} A_{11}. \quad (28)$$

$\mathbb{T}_1$  can be measured in terms of two new observables  $A_{10}$  and  $A_{11}$ , defined in terms of angular asymmetries as follows:

$$A_{10} = \frac{\int_0^{2\pi} d\phi \int_0^1 d\cos\theta_K \left[ \int_{-1}^{-1/2} - \int_{-1/2}^{1/2} + \int_{1/2}^1 \right] d\cos\theta_{\ell} \frac{d^4(\Gamma + \bar{\Gamma})}{dq^2 d\cos\theta_{\ell} d\cos\theta_K d\phi}}{\int_0^{2\pi} d\phi \int_{-1}^1 d\cos\theta_K \int_{-1}^1 d\cos\theta_{\ell} \frac{d^4(\Gamma + \bar{\Gamma})}{dq^2 d\cos\theta_{\ell} d\cos\theta_K d\phi}}, \quad (29)$$

$$A_{11} = \frac{\int_0^{2\pi} d\phi \left[ \int_{-1}^{-1/2} - \int_{-1/2}^{1/2} + \int_{1/2}^1 \right] d\cos\theta_K \left[ \int_{-1}^{-1/2} - \int_{-1/2}^{1/2} + \int_{1/2}^1 \right] d\cos\theta_{\ell} \frac{d^4(\Gamma + \bar{\Gamma})}{dq^2 d\cos\theta_{\ell} d\cos\theta_K d\phi}}{\int_0^{2\pi} d\phi \int_{-1}^1 d\cos\theta_K \int_{-1}^1 d\cos\theta_{\ell} \frac{d^4(\Gamma + \bar{\Gamma})}{dq^2 d\cos\theta_{\ell} d\cos\theta_K d\phi}} \quad (30)$$

If the two asymmetries  $A_{10}$  and  $A_{11}$  are measured experimentally then we can experimentally obtain the correction term arising due to lepton masses.

In the absence of a measurement of  $A_{10}$  and  $A_{11}$ , we estimate  $\mathbb{T}_1$  using the factor values evaluated in Ref. [6]. The effect of adding mass of the lepton is thus, easily incorporated by the following substitutions:

$$\zeta \rightarrow \beta^2 \zeta \quad (31)$$

$$u_{\lambda}^2 \rightarrow \beta^2 u_{\lambda}^2 \quad (32)$$

$$F_{\lambda} \rightarrow F_{\lambda} - \frac{\mathbb{T}_1}{\Gamma_f} \quad (33)$$

We have incorporated the effect of finite mass corrections as given in the above equations.

#### IV. DETAILS OF $\chi^2$ FIT TO THE PARAMETERS

In this section we discuss the details of  $\chi^2$  fit after including complex contributions of the amplitudes and considering systematic uncertainty arising mainly due to bin average effect. It is shown in Ref. [1] that  $\varepsilon_\lambda$ 's contribute to the helicity fractions  $F_\lambda$  and asymmetry  $A_4$ . Using the bin average central values of  $\varepsilon_\lambda/\sqrt{\Gamma_f}$ , with  $\pm 1\sigma$  errors from Table. I we can numerically separate out the complex contributions from experimental measured values of the observables. We calculate the central value with  $\pm 1\sigma$  error of the modified observables  $F_\lambda^{\text{ex}'}$  and  $A_4^{\text{ex}'}$  given by,

$$F_\lambda^{\text{ex}'} = F_\lambda^{\text{ex}} - \frac{2\varepsilon_\lambda^2}{\Gamma_f}, \quad (34)$$

$$A_4^{\text{ex}'} = A_4^{\text{ex}} - \frac{2\sqrt{2}\varepsilon_0\varepsilon_\parallel}{\pi\Gamma_f}, \quad (35)$$

which enter in the  $\chi^2$  definition Eq. (36) below. It enables us to take into account the complex corrections in our analysis and extract out the variables  $P_1$ ,  $P_2$ ,  $\zeta$ ,  $u_0$  and  $u_\perp$  (which only deal with the real part of amplitude) from experimental measurements of the observables accurately. It should be noted that Eqs. (9)-(13) of the main paper are valid for each  $q^2$  point. Thus a fit with bin average values of the observables may lead to a biased conclusion. To avoid this issue we have added systematic uncertainties for each observables due to bin average effect with the introduction of new parameter  $\beta$ , where the change in each observable  $\mathcal{O}$  is given by,

$$\mathcal{O} \rightarrow \mathcal{O} + \beta \mathcal{O}^s.$$

$\mathcal{O}^s$  is the maximum shift for each observables from a best fitted  $q^2$  function to 14 bin LHCb data [3] within the concerned bin interval. The details of  $\mathcal{O}^s$  evaluation are highlighted in Fig. 2 where red error bars are LHCb measurements and gray curves represent best fitted polynomial in  $q^2$  for 14 bin LHCb data. We use 14 bin measurement (based on the method of moments [4]) from LHCb to fit the polynomial in  $q^2$ , rather than the 8 bin data set as it provides more information to determine the shape of the polynomial for entire  $q^2$  region. The black dashed line denotes the maximum deviation of bin average central value of the observable from the  $q^2$  function for the region  $6 \leq q^2 \leq 8 \text{ GeV}^2$  and  $\mathcal{O}^s$  is the length of the line for observable  $\mathcal{O}$ . Similar technique is applied for other  $q^2$  bins also and the values of systematic errors are given in Table. II for all observables. Therefore the  $\chi^2$  definition is

$$\chi^2 = \left[ \left( \frac{F_\perp^{\text{ex}'} - F_\perp - \beta F_\perp^s}{\Delta F_\perp^{\text{ex}'}} \right)^2 + \left( \frac{F_L^{\text{ex}'} - F_L - \beta F_L^s}{\Delta F_L^{\text{ex}'}} \right)^2 + \left( \frac{A_4^{\text{ex}'} - A_4 - \beta A_4^s}{\Delta A_4^{\text{ex}'}} \right)^2 \right. \\ \left. + \left( \frac{A_{\text{FB}}^{\text{ex}} - A_{\text{FB}}^2 - \beta A_{\text{FB}}^{2s}}{2A_{\text{FB}}^{\text{ex}}\Delta A_{\text{FB}}^{\text{ex}}} \right)^2 + \left( \frac{A_5^{\text{ex}} - A_5^2 - \beta A_5^{2s}}{2A_5^{\text{ex}}\Delta A_5^{\text{ex}}} \right)^2 + \beta^2 \right], \quad (36)$$

where  $A_{\text{FB}}^{\text{ex}}$  and  $A_5^{\text{ex}}$  indicate experimental central values of the observables  $A_{\text{FB}}$  and  $A_5$  with  $\pm 1\sigma$  errors as  $\Delta A_{\text{FB}}^{\text{ex}}$  and  $\Delta A_5^{\text{ex}}$ , respectively. Similarly  $F_\perp^{\text{ex}'}$ ,  $F_L^{\text{ex}'}$  and  $A_4^{\text{ex}'}$  are the central values of the modified observables defined in Eqs. (34) and (35) and  $\Delta F_\perp^{\text{ex}'}$ ,  $\Delta F_L^{\text{ex}'}$ ,  $\Delta A_4^{\text{ex}'}$  are  $\pm 1\sigma$  uncertainties in it. The systematic uncertainties added for each observables are denoted as  $F_\perp^s$ ,  $F_L^s$ ,  $A_4^s$ ,  $A_{\text{FB}}^{2s}$ ,  $A_5^{2s}$  and these values are quoted in Table. II. The observables  $F_\perp$ ,  $F_L$ ,  $A_4$ ,  $A_{\text{FB}}^2$  and  $A_5^2$  are evaluated in terms of the five parameters  $P_1$ ,  $P_2$ ,  $\zeta$ ,  $u_0$  and  $u_\perp$  using Eqs. (9)–(13) of the main paper. Considering the inverse of the covariance matrix the error ellipsoids are constructed for all the eight bins corresponding to the  $q^2$  values in the range  $(0.1 - 0.98) \text{ GeV}^2$ ,  $(1.1 - 2.5) \text{ GeV}^2$ ,  $(2.5 - 4.0) \text{ GeV}^2$ ,  $(4 - 6) \text{ GeV}^2$ ,  $(6 - 8) \text{ GeV}^2$ ,  $(11.0 - 12.5) \text{ GeV}^2$ ,  $(15 - 17) \text{ GeV}^2$  and  $(17 - 19) \text{ GeV}^2$ . It can be seen that  $\beta$  is treated as a nuisance parameter with values varying between +1 and -1. The  $\chi^2$  function is minimized w.r.t six parameters  $P_1$ ,  $P_2$ ,  $\zeta$ ,  $u_0$ ,  $u_\perp$  and  $\beta$  and the contours shown in Fig. 1 and Fig. 2 are the allowed regions in the corresponding planes. The best fitted values with  $\pm 1\sigma$  errors of the parameter  $\beta$  for all eight bins are  $7.4 \times 10^{-5} \pm 0.015$ ,  $1.6 \times 10^{-5} \pm 0.020$ ,  $0.153 \pm 0.011$ ,  $1.0 \times 10^{-17} \pm 0.005$ ,  $0.736 \pm 0.020$ ,  $0.251 \pm 0.003$ ,  $0.261 \pm 0.001$  and  $0.161 \pm 0.012$ , respectively.

It should be noted that as discussed in Sec. III finite lepton mass can affect the analysis in the first two  $q^2$  region namely  $q^2 \leq 2.5 \text{ GeV}^2$  and in the absence of a measurement of  $A_{10}$  and  $A_{11}$  we have to rely on some hadronic estimates. This in principle may induce more uncertainties and we took a conservative approach by considering two times the  $\mathcal{O}^s$  values for all observables given in Table. II for the two bins  $0.1 \leq q^2 \leq 0.98 \text{ GeV}^2$  and  $1.1 \leq q^2 \leq 2.5 \text{ GeV}^2$ .

| $q^2$ range in $\text{GeV}^2$ | $F_{\perp}^s$ | $F_L^s$ | $A_4^s$ | $A_{\text{FB}}^{2s}$ | $A_5^{2s}$ |
|-------------------------------|---------------|---------|---------|----------------------|------------|
| $0.1 \leq q^2 \leq 0.98$      | 0.014         | 0.230   | 0.088   | 0.002                | 0.016      |
| $1.1 \leq q^2 \leq 2.5$       | 0.223         | 0.151   | 0.036   | 0.034                | 0.010      |
| $2.5 \leq q^2 \leq 4.0$       | 0.164         | 0.223   | 0.064   | 0.013                | 0.004      |
| $4.0 \leq q^2 \leq 6.0$       | 0.069         | 0.138   | 0.021   | 0.002                | 0.008      |
| $6.0 \leq q^2 \leq 8.0$       | 0.132         | 0.165   | 0.028   | 0.020                | 0.019      |
| $11.0 \leq q^2 \leq 12.5$     | 0.029         | 0.063   | 0.006   | 0.051                | 0.023      |
| $15.0 \leq q^2 \leq 17.0$     | 0.019         | 0.048   | 0.027   | 0.036                | 0.023      |
| $17.0 \leq q^2 \leq 19.0$     | 0.109         | 0.020   | 0.039   | 0.077                | 0.053      |

TABLE II. The systematic uncertainties for each observables  $F_{\perp}$ ,  $F_L$ ,  $A_4$ ,  $A_{\text{FB}}^2$  and  $A_5^2$  are shown. The values denote magnitude of maximum deviation of the bin average central value from the fitted  $q^2$  polynomial within every  $q^2$  bin.

We emphasize that resonances in our analysis will only affect the fitted function in  $q^2$ , which in turn will induce more systematic uncertainties to the observables. We have checked our chi-square fit by increasing the systematic uncertainties (twice the values given in Table-II of supplementary material) for the regions  $11 \leq q^2 \leq 12.5 \text{ GeV}^2$  and  $15 \leq q^2 \leq 17 \text{ GeV}^2$  and our results are stable with it.

The deviations in the hadronic parameters  $P_1$ ,  $P_2$  and  $\zeta$  are calculated by defining a chi-square function

$$\chi'^2 = \frac{(\mathcal{P}_{\text{SM}} - \mathcal{P}_{\text{Fit}})^2}{\delta\mathcal{P}_{\text{SM}}^2 + \delta\mathcal{P}_{\text{Fit}}^2} \quad (37)$$

where  $\mathcal{P}_{\text{SM}}$  and  $\mathcal{P}_{\text{Fit}}$  denote the SM predictions and the best fit values from experimental data respectively and  $\delta\mathcal{P}_{\text{SM}}^2$  and  $\delta\mathcal{P}_{\text{Fit}}^2$  are the corresponding uncertainties in the parameters  $P_1$ ,  $P_2$  and  $\zeta$ . Below in the Table. III, we show the  $\chi'^2$  values with the deviations expressed in terms of statistical confidence level. The fits for the values of  $V$ ,  $A_1$  and  $A_2$  are given in Table. I of the paper.

| $q^2$ range in $\text{GeV}^2$ | $P_1$                  | $P_2$                    | $\zeta$               |
|-------------------------------|------------------------|--------------------------|-----------------------|
| $0.1 \leq q^2 \leq 0.98$      | 0.35                   | 93.32 ( $\geq 9\sigma$ ) | 4.15 ( $2.04\sigma$ ) |
| $1.1 \leq q^2 \leq 2.5$       | 1.22                   | 4.93( $2.22\sigma$ )     | 5.74 ( $2.40\sigma$ ) |
| $2.5 \leq q^2 \leq 4.0$       | 0.55                   | 1.65                     | 3.24                  |
| $4.0 \leq q^2 \leq 6.0$       | 0.43                   | 0.07                     | 1.35                  |
| $6.0 \leq q^2 \leq 8.0$       | 17.68 ( $4.21\sigma$ ) | 0.59                     | 1.30                  |
| $11.0 \leq q^2 \leq 12.5$     | 26.79 ( $5.18\sigma$ ) | 22.65 ( $4.76\sigma$ )   | 7.77 ( $2.79\sigma$ ) |
| $15.0 \leq q^2 \leq 17.0$     | 30.64 ( $5.54\sigma$ ) | 28.52 ( $5.34\sigma$ )   | 2.97                  |
| $17.0 \leq q^2 \leq 19.0$     | 0.93                   | 0.15                     | 0.41                  |

TABLE III. The  $\chi'^2$  values for  $P_1$ ,  $P_2$  and  $\zeta$ . Significant standard deviation are also depicted in round brackets.

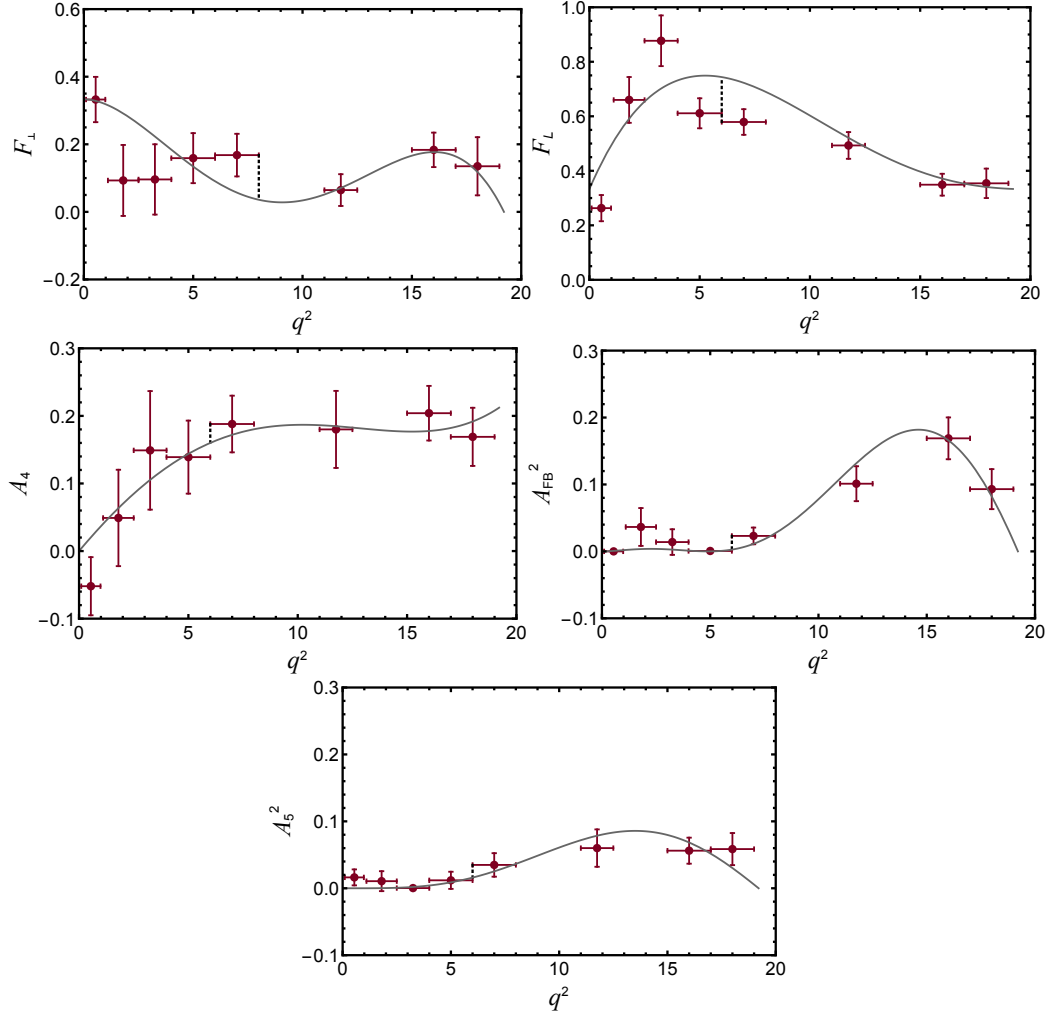

FIG. 2. (color online). The procedure to calculate systematic errors are shown for observables  $F_{\perp}$ ,  $F_L$ ,  $A_4$ ,  $A_{\text{FB}}^2$  and  $A_5^2$ , respectively. The red error bars are LHCb measurements and gray curves represent best fitted polynomial in  $q^2$  for 14 bin LHCb data [3]. The black dashed lines denote the maximum deviation of bin average central value of the observables with the  $q^2$  function for bin  $6 \leq q^2 \leq 8 \text{ GeV}^2$ . The length of these black lines are denoted by  $F_{\perp}^s$ ,  $F_L^s$ ,  $A_4^s$ ,  $A_{\text{FB}}^{2s}$  and  $A_5^{2s}$ , respectively. Similar lines can be drawn for other  $q^2$  bins also and the values of systematic errors are given in Table. II for all observables.

## V. TESTING OBSERVABLES USING THE RELATION BETWEEN OBSERVABLES.

In Refs. [1, 7] a relation depending purely on observables was derived. If  $\varepsilon_\lambda$  are small and ignored, the relation is exact and given in Eq. (16) of the paper we can use it to solve for any of the observables. A solution for  $A_4$  is

$$A_4 = \frac{8A_5A_{\text{FB}}}{9\pi F_\perp} + \frac{\sqrt{4F_\parallel F_\perp - \frac{16}{9}A_{\text{FB}}^2} \sqrt{4F_L F_\perp - \frac{32}{9}A_5^2}}{2\sqrt{2}\pi F_\perp}. \quad (38)$$

Whereas, the solution for  $A_5$  and  $A_{\text{FB}}$  are given by,

$$A_5 = \frac{\pi A_4 A_{\text{FB}}}{2F_\parallel} \pm \frac{\sqrt{(\frac{9}{4}F_\parallel F_\perp - A_{\text{FB}}^2)(2F_\parallel F_L - \pi^2 A_4^2)}}{2F_\parallel} \quad (39)$$

$$A_{\text{FB}} = \frac{\pi A_4 A_5}{F_L} \pm \frac{\sqrt{(\frac{9}{8}F_L F_\perp - A_5^2)(2F_\parallel F_L - \pi^2 A_4^2)}}{F_L}. \quad (40)$$

It may noted that Eqs. (38), (39) and (40) depend only on observables and not on any theoretical parameters. This is the advantage of the  $B \rightarrow K^* \ell^+ \ell^-$  mode. The solutions for  $A_5$  and  $A_{\text{FB}}$  have ambiguities. We chose the ambiguity for which the chi-squared deviations are the least.

We generate a set of events for every bin, with each event consisting of randomly chosen values drawn from Gaussian distributions generated for each of the observables  $F_L$ ,  $F_\perp$ ,  $A_4$ ,  $A_5$ ,  $A_{\text{FB}}$ . The distributions are generated using experimental results from Ref. [2], with the experimentally measured value as mean and the uncertainty as standard deviation. To generate the distribution of  $A_4$  events in a given  $q^2$  bin we use Eq. (38) and the values of the other observables  $F_L$ ,  $F_\perp$ ,  $A_5$  and  $A_{\text{FB}}$ . The values of  $A_4$  obtained are compared with the experimental values. The result is shown in Fig. 3.

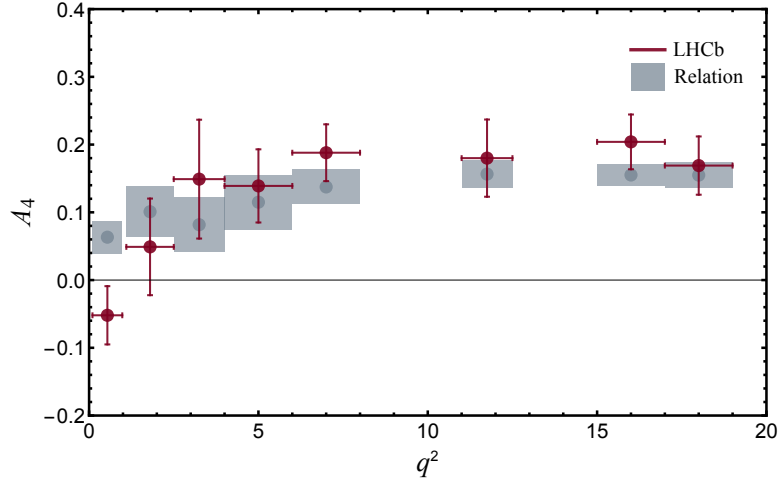

FIG. 3. The mean values and  $1\sigma$  uncertainty bands for  $A_4$  calculated using using Eq. (38) are shown in gray bands. The error bars in red (dark) correspond to the experimentally measured central values and errors in  $A_4$  for the respective  $q^2$  bins.

In a way similar to  $A_4$  the distributions  $A_{\text{FB}}$  can also be generated. Such a distribution for  $A_{\text{FB}}$  is presented in 4. Finally, we also present the distribution for  $A_5$  and  $P_5'$  in Fig. 5.

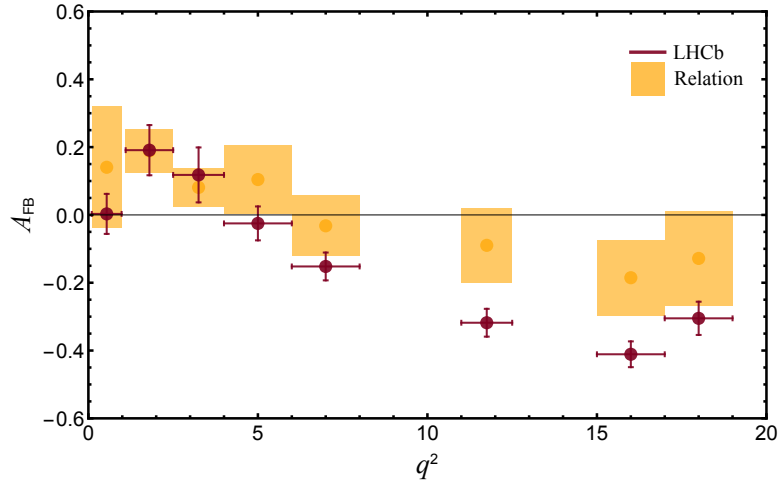

FIG. 4. The mean values and  $1\sigma$  uncertainties for  $A_{FB}$  calculated using Eq. (40) are shown by yellow bands. The error bars in red (dark) correspond to the experimentally measured central values and errors in  $A_{FB}$  for the respective  $q^2$  bins. See text for details.

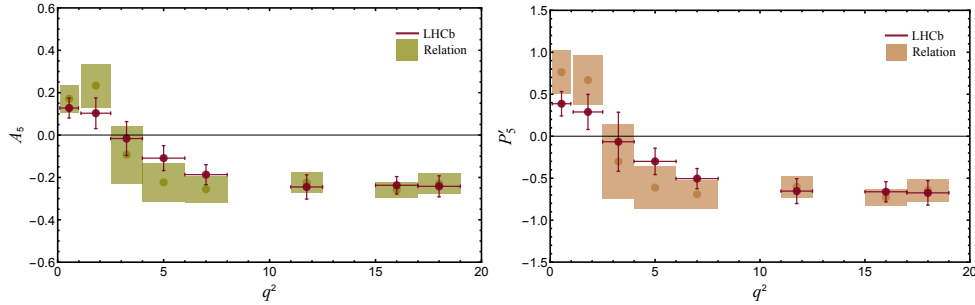

FIG. 5. (color online). The mean values and  $1\sigma$  uncertainties for  $A_5$  calculated using Eq. (39) are shown by green bands in the figure on the left. Similar mean values and  $1\sigma$  uncertainties for  $P'_5$  are depicted by light brown bands in the figure on the right. The error bars in red (dark) correspond to the experimentally measured central values and errors in  $A_5$  and  $P'_5$  respectively for the various  $q^2$  bins.

The chi-square values for the four asymmetries  $A_{FB}$ ,  $A_4$ ,  $A_5$  and  $P'_5$  for entire  $q^2$  region are shown in Table V. When a deviation of order  $2\sigma$  or more was observed the simulations were repeated several times to ensure the discrepancy is not statistical in nature. The values for the observable  $A_{FB}$  in 6th and 7th bins are the average chi-square value for thousand  $A_{FB}$  distributions. In the calculation of  $A_4$  the effects of  $\epsilon_\lambda$ 's was also studied. In the first bin the chi-square value for  $A_4$  is the average over ten  $A_4$  distributions because of the huge computational time after including finite lepton mass effect and complex contribution of the amplitudes ( $\epsilon_\lambda$ 's) in the programming.

- 
- [1] R. Mandal, R. Sinha and D. Das, Phys. Rev. D **90**, no. 9, 096006 (2014) [arXiv:1409.3088 [hep-ph]].
  - [2] The LHCb Collaboration [LHCb Collaboration], CERN-LHCb-CONF-2015-002.
  - [3] R. Aaij *et al.* [LHCb Collaboration], JHEP **1602**, 104 (2016), [arXiv:1512.04442 [hep-ex]].
  - [4] F. Beaujean, M. Chrzaszcz, N. Serra and D. van Dyk, Phys. Rev. D **91**, 114012 (2015)
  - [5] W. Altmannshofer, P. Ball, A. Bharucha *et al.*, JHEP **0901**, 019 (2009). [arXiv:0811.1214 [hep-ph]].
  - [6] A. Bharucha, D. M. Straub and R. Zwicky, arXiv:1503.05534 [hep-ph].
  - [7] D. Das and R. Sinha, Phys. Rev. D **86** (2012) 056006 [arXiv:1205.1438 [hep-ph]];

| $q^2$ range in $\text{GeV}^2$ | $A_{\text{FB}}$      | $A_4$                | $A_5$ | $P'_5$ |
|-------------------------------|----------------------|----------------------|-------|--------|
| $0.1 \leq q^2 \leq 0.98$      | 0.53                 | 5.20 (2.3 $\sigma$ ) | 0.30  | 1.58   |
| $1.1 \leq q^2 \leq 2.5$       | 0.00                 | 0.38                 | 1.08  | 1.10   |
| $2.5 \leq q^2 \leq 4.0$       | 0.14                 | 0.54                 | 0.23  | 0.18   |
| $4.0 \leq q^2 \leq 6.0$       | 1.33                 | 0.13                 | 1.11  | 1.11   |
| $6.0 \leq q^2 \leq 8.0$       | 1.50                 | 1.07                 | 0.77  | 0.80   |
| $11.0 \leq q^2 \leq 12.5$     | 4.44 (2.1 $\sigma$ ) | 0.14                 | 0.08  | 0.07   |
| $15.0 \leq q^2 \leq 17.0$     | 3.12 (1.8 $\sigma$ ) | 1.21                 | 0.16  | 0.19   |
| $17.0 \leq q^2 \leq 19.0$     | 1.42                 | 0.08                 | 0.03  | 0.03   |

TABLE IV. The  $\chi^2$  values for  $A_{\text{FB}}$ ,  $A_4$ ,  $A_5$  and  $P'_5$ . Significant standard deviation are also depicted in round brackets. It can be seen that  $A_5$  and  $P'_5$  are in excellent agreement.
